# Supplementary material for: Communication-Efficient Variance-Reduced Decentralized Stochastic Optimization over Time-Varying Directed Graphs
Source: arXiv:2101.09583 source file (2021-12-02)
Supplement: Supplementary file 1 [file tac_appendix.tex]

% Let $\Tilde{\nabla f_i(\z_i^t)}=\nabla f_{im}(\z_i^t)-\nabla f_{im}(\Tilde{w}_{i})+\Tilde{\mu} $ be gradient term in SVRG algorithm. 

The main focus of the appendix is the proof of the claims of Theorem~1, i.e., establishing linear convergence of Algorithm \ref{alg:B}. This will require several auxiliary results stated as lemmas whose proofs are provided in the supplementary material. Specifically, the appendix starts the proof with the following three lemmas: in Lemma~2, we state an upper bound on the consensus error, i.e., the difference between {\color{blue}{local}} vectors and the average vectors,
{\color{blue}{at a time step which is a multiple of $\mathcal{B}$, } } $E[|z_{im}^{(k+1)\mathcal{B}}-\Bar{z}_{m}^{(k+1)\mathcal{B}} |^2]$; in Lemma~3, we provide an upper bound on the optimality gap, i.e., the difference between average vectors and the optimal vector, $E[\|\Bar{\z}^{(k+1)\mathcal{B}} - \x^* \|^2]$; in Lemma~4, we upper bound the gradient tracking error, i.e., the error on the gradient and the averaged gradient. 

% in Lemma~4-6, we further compute upper bounds for the gradient terms in Lemma~2-3; finally, in Lemma~7-9, we formulate a linear system and show the linear convergence rate. 
\newtheorem*{lemma2}{Lemma $2$}
\begin{lemma2}
Suppose each component of local objective function $f_{i, j}$ is $L$-smooth. The updates generated by Algorithm \ref{alg:B} satisfy
$\forall i \leq n, k \geq 0, 0 < m \leq d$, 
\begin{equation}
\begin{aligned}
    E[|z_{im}^{(k+1)\mathcal{B}}-\Bar{z}_{m}^{(k+1)\mathcal{B}} |^2] & \leq \frac{1+\sigma^2}{2}E[|z_{im}^{k\mathcal{B}}-\Bar{z}_{m}^{k\mathcal{B}} |^2 ] \\ & \quad +\frac{2\alpha^2}{1-\sigma^2}E[|g_{im}^{k\mathcal{B}}-\Bar{g }_{m}^{k\mathcal{B}} \|^2 ]
\end{aligned}
\end{equation}
\end{lemma2}

Before Lemma~3 and 4, for $k \geq 0$, we first denote 
\begin{equation}
    \Bar{\tau}^{k\mathcal{B}} = \frac{1}{n}\sum_{i=1}^n \tau_i^{k\mathcal{B}}
\end{equation}
 and 
\begin{equation}
    \tau_i^{(k+1)\mathcal{B}} = \begin{cases}
    \x_i^{(k+1)\mathcal{B}} & \mathrm{if} \quad (k+1)\mathcal{B} \mod T = 0 \\
    \x_i^{k\mathcal{B}} & \mathrm{otherwise}.
    \end{cases}
\end{equation}

\newtheorem*{lemma3}{Lemma $3$}
\begin{lemma3}
Suppose the above assumptions {\color{green} Abolfazl: which assumptions? you mean notations? be specific} hold and $f$ is $\mu$-strongly-convex.  
Let $0 < \alpha < \frac{1}{L}$ where $L$ is the smoothness parameter for local objectives $f_{i, j}$ and then $\forall\ k>0$:
\begin{equation}
\begin{aligned}
    E[\|\Bar{\z}^{(k+1)\mathcal{B}} - \x^* \|^2] & \leq \frac{L^2\alpha}{n\mu} E[\sum_{i=1}^n  \|\Bar{\z}^{k\mathcal{B}}-\z_i^{k\mathcal{B}} \|^2 ] \\ & \quad + (1-\mu \alpha)E[\|\Bar{\z}^{k\mathcal{B}}-\x^* \|^2]\\
    &\quad + \frac{\alpha^2}{n^2}(4L^2\sum_{i=1}^n \|\x_i^{k\mathcal{B}} -\Bar{\z}^{k\mathcal{B}} \|^2 \\ & \quad + 4L^2\sum_{i=1}^nE[n \|\tau_i^{k\mathcal{B}} -\Bar{\tau}^{k\mathcal{B}} \|^2]\\ & \quad + 4L^2 E[n\|\Bar{\tau}^{k\mathcal{B}} - \x^* \|^2])
\end{aligned}
\end{equation}
\end{lemma3}

\newtheorem*{lemma4}{Lemma $4$}
\begin{lemma4}
Suppose that the above assumptions hold {\color{green} Abolfazl: which assumptions? be specific}, $f$ is $\mu$-strongly-convex and the local objectives $f_{i, j}$ are $L$-smooth, then
\begin{equation}
\begin{aligned}
& E[\frac{\sum_{m=1}^d \sum_{i=1}^n \|g_{im}^{(k+1)\mathcal{B}}-\Bar{g}_m^{(k+1)\mathcal{B}} \|^2  }{L^2}\\ & \leq \frac{120}{1-\sigma^2}E[\sum_{i=1}^n  \|\Bar{\z}^{k\mathcal{B}}-\z_i^{k\mathcal{B}} \|^2  ]\\& \quad + \frac{88}{1-\sigma^2}E[ n\|\Bar{\z}^{k\mathcal{B}}-\x^* \|^2] \\& \quad + \frac{3+\sigma^2}{4} E[\frac{\sum_{m=1}^d \sum_{i=1}^n \|g_{im}^{k\mathcal{B}}-\Bar{g}_m^{k\mathcal{B}} \|^2  }{L^2} ]\\ & \quad + \frac{38}{1-\sigma^2} E[\sum_{i=1}^n  \|\Bar{\z}^{k\mathcal{B}}-\z_i^{k\mathcal{B}} \|^2  ] \\ & \quad
+ \frac{38}{1-\sigma^2} E[n \|\Bar{\tau}^{k\mathcal{B}} - \x^* \|^2 ]
\end{aligned}
\end{equation}
\end{lemma4}

With the upper bounds in Lemma~2, 3 and 4 showing recursive relationship concerning the terms on the consensus error, optimality error and gradient tracking error,
we can summarize to formulate a linear dynamic system.
To explicitly derive the linear convergence rate, we will establish the converging property of the system and further the vanishing optimality gap. Specifically, we define 
\begin{equation}
    \u^{k\mathcal{B}} = \begin{bmatrix}
    E[\sum_{i=1}^n  \|\Bar{\z}^{k\mathcal{B}}-\z_i^{k\mathcal{B}} \|^2  ] \\
    E[ n\|\Bar{\z}^{k\mathcal{B}}-\x^* \|^2] \\
    E[\frac{\sum_{m=1}^d \sum_{i=1}^n \|g_{im}^{k\mathcal{B}}-\Bar{g}_m^{k\mathcal{B}} \|^2  }{L^2} ]
    \end{bmatrix}
\end{equation}

\begin{equation}
    \Tilde{\u}^{k\mathcal{B}} = \begin{bmatrix}
     E[\sum_{i=1}^n \| \tau_i^{k\mathcal{B}}-\Bar{\tau}^{k\mathcal{B}} \|^2 ] \\
     E[n \|\Bar{\tau}^{k\mathcal{B}} - \x^* \|^2 ] \\
     \mathbf{0}
    \end{bmatrix}
\end{equation}

\begin{equation}
    J_{\alpha} = \begin{bmatrix}
    \frac{1+\sigma^2}{2} & 0 & \frac{2\alpha^2L^2}{1-\sigma^2} \\
    \frac{2L^2\alpha}{\mu} & 1-\frac{\mu \alpha}{2} & 0 \\
    \frac{120}{1-\sigma^2} & \frac{88}{1-\sigma^2} & \frac{3+\sigma^2}{4} 
    \end{bmatrix}
\end{equation}

\begin{equation}
    H_{\alpha} = \begin{bmatrix}
    0 & 0 & 0 \\
    \frac{4L^2 \alpha^2}{n} & \frac{4L^2 \alpha^2}{n} & 0 \\
    \frac{38}{1-\sigma^2} & \frac{38}{1-\sigma^2} & 0
    \end{bmatrix}
\end{equation}
and then state the interrelationship of the linear system in Proposition~1. 

\newtheorem*{proposition1}{Proposition $1$}
\begin{proposition1}
Suppose the assumptions above hold, the objective function $f$ is $\mu$-strongly-convex and each component of local objective function $f_{i, j}$ is $L$-smooth. If $0 \leq \alpha \leq \frac{\mu(1-\sigma^2)}{14\sqrt{2}L^2}$, 
$\forall k \geq 0$,
\begin{equation}
    \u^{(k+1)\mathcal{B}} \leq J_{\alpha}\u^{k\mathcal{B}} + H_{\alpha} \Tilde{\u}^{k\mathcal{B}}
\end{equation}
\end{proposition1}

Then for the inner loop, $\forall k \in [s\lfloor T/ \mathcal{B} \rfloor, (s+1)\lfloor T/ \mathcal{B} \rfloor-1]$
\begin{equation}
    \u^{(k+1)\mathcal{B}} \leq J_{\alpha}\u^{k\mathcal{B}} + H_{\alpha} \u^{sT}
\end{equation}

For the outer loop, $\forall s \geq 0$
\begin{equation}
    \u^{(s+1)T} \leq (J_{\alpha}^T + \sum_{l=0}^{T-1}J_{\alpha}^l H_{\alpha}) \u^{sT}
\end{equation}

To guarantee the linear decay of the outer loop sequence, we compute the range of the inner loop length $T$ and the step size $\alpha$ such that the system is converging by requiring
\begin{equation}
    \rho(J_{\alpha}^T + \sum_{l=0}^{T-1}J_{\alpha}^l H_{\alpha} ) < 1
\end{equation}
In the following Lemma~5 and 6, we derive the range of $\alpha$ such that the weighted matrix norm of $J_{\alpha}^T$ and $ \sum_{l=0}^{T-1}J_{\alpha}^l H_{\alpha}$ are small. 
\newtheorem*{lemma5}{Lemma $5$}
\begin{lemma5}\label{lemma5}
% Refer to lemma $11$ in GT-SVRG
Suppose the assumptions above hold, the objective function $f$ is $\mu$-strongly-convex and each component of local objective function $f_{i, j}$ is $L$-smooth.
Suppose that $ 0 < \alpha \leq \frac{(1-\sigma^2)^2}{187\Tilde{Q}L}$ where $\Tilde{Q} = \frac{L}{\mu}$.
Let $\mathbf{\delta} = \begin{bmatrix}
1, 8\Tilde{Q}^2, \frac{6592\Tilde{Q}^2}{(1-\sigma^2)^2}
\end{bmatrix}$,
and finally we have that
\begin{equation}
    \rho(J_{\alpha}) < \| |J_{\alpha}| \|^{\mathbf{\delta}}_{\infty} < 1 - \frac{\mu \alpha}{4}
\end{equation}
\end{lemma5}

\newtheorem*{lemma6}{Lemma $6$}
\begin{lemma6}\label{lemma6}
% Refer to lemma $12$ in GT-SVRG
Suppose the assumptions above hold, the objective function $f$ is $\mu$-strongly-convex and each component of local objective function $f_{i, j}$ is $L$-smooth.
If $ 0 < \alpha \leq \frac{(1-\sigma^2)^2}{187\Tilde{Q}L}$, then 
\begin{equation}
    \| |\sum_{l=0}^{T-1}J_{\alpha}^l H_{\alpha}| \|^{\q}_{\infty} \leq
     \| | (I_3 - J_{\alpha})^{-1} H_{\alpha} | \|^{\q}_{\infty}< 0.66
\end{equation}
where $\q = [1, 1, \frac{1453}{(1-\sigma^2)^2}]$. 
\end{lemma6}

Combining Lemma~5 and 6, we appropriately select values of $T$ and $\alpha$ to prove the linear decay of the outer loop sequence in Lemma~7 to complete the proof of Theorem~1.

\newtheorem*{lemma7}{Lemma $7$}
\begin{lemma7}\label{lemma7}
If the step size $\alpha = \frac{(1-\sigma^2)^2}{187\Tilde{Q}L}$, the number of inner-loop $ T = \mathcal{B} \lceil \frac{748\Tilde{Q}^2}{(1-\sigma^2)^2 \mathcal{B}}\log (200\Tilde{Q}^2) \rceil $, then
\begin{equation}
    \|\u^{(s+1)T}\|_{\infty}^{\q} \leq 0.7\|\u^{sT}\| _{\infty}^{\q}  
\end{equation}
where $\q = [1, 1, \frac{1453}{(1-\sigma^2)^2}]$. 
\end{lemma7}

The lemma implies that for the outer loop of Algorithm \ref{alg:B} to reach $\epsilon$-accuracy, the algorithm needs to run at most $\O(\frac{\Tilde{Q}^2\ln \Tilde{Q}}{(1-\sigma^2)^2}\ln 1/\epsilon)$ communication rounds. In the process, the gradient needs to be computed $\O(\frac{\Tilde{Q}^2\ln \Tilde{Q}}{(1-\sigma^2)^2\mathcal{B}}\ln 1/\epsilon)$ times.
Therefore, we complete the proof of Theorem~1.

%{\color{blue}{Move to one-column tac supplementary.tex file.}}
